# Supplementary material for: Automated Verification of Soundness of DNN Certifiers
Source: arXiv:2504.04542 source file (2025-04-06)
Supplement: Supplementary file 1 [file absiproofs.tex]

\section{Proofs for Lemmas in Sections~\ref{sec:background} and \ref{sec:overview}}
\label{appendix:bgroundproofs}
\begin{lemma}
% \label{lem:redsound}
$f^\sharp$ is sound w.r.t a deterministic function $f$ iff  $\ \forall a \in \mathcal{A}, f(\gamma(a)) \subseteq \gamma(f^\sharp(a))$. 
    % If $f$ is deterministic for all inputs to the DNN, and $\forall a \in \mathcal{A}, f(\gamma(a)) \subseteq \gamma(f^\sharp(a))$, then, $f^\sharp$ is sound w.r.t $f$.
\end{lemma}
\begin{proof}
    $f^\sharp$ is sound w.r.t $f$ :  
    $\forall a \in \mathcal{A} \cdot \forall c \in \mathcal{C} \cdot c \subseteq \gamma(a) \implies f(c) \subseteq \gamma(f^\sharp(a)) $
    \begin{enumerate}
        \item Let $f^\sharp$ be sound w.r.t $f$ \\
        So, $\forall a \in \mathcal{A} \cdot \forall c \in \mathcal{C} \cdot c \subseteq \gamma(a) \implies f(c) \subseteq \gamma(f^\sharp(a)) $ \\ 
        Let $c = \gamma(a)$ \\ 
        $\implies f(\gamma(a)) \subseteq \gamma(f^\sharp(a))$ \\  

        \item Since $f$ is deterministic and $c$ is a set of inputs to the DNN, so, $f$ is monotonic w.r.t $\subseteq$ ordering. \\
        So, $c_1 \subseteq c_2 \implies f(c_1) \subseteq f(c_2)$ \\
        Given that $\forall a \in \mathcal{A}, f(\gamma(a)) \subseteq \gamma(f^\sharp(a))$ \\ 
        Let $c \subseteq \gamma(a)$ \\ 
        $\implies f(c) \subseteq f(\gamma(a))$ \\ 
        $\implies f(c) \subseteq f(\gamma(a)) \subseteq \gamma(f^\sharp(a))$ \\ 
        $\implies f(c) \subseteq \gamma(f^\sharp(a))$ \\
        Hence, $f^\sharp$ is sound w.r.t $f$.
    \end{enumerate}
\end{proof}

\begin{lemma}
    If $f_1^\sharp$ and $f_2^\sharp$ are sound w.r.t $f_1$ and $f_2$ respectively, then, $f_1^\sharp \circ f_2^\sharp$ is sound w.r.t $f_1 \circ f_2$.
\end{lemma}
% \begin{proof} 
% Let, $c \in \mathcal{C}, a \in \mathcal{A}$ s.t., $c\subseteq \gamma(a)$. Since $f^\sharp_1$ is sound, $f_1(c) \subseteq \gamma(f^\sharp_1(a))$. \\
% Let $c' \subseteq \gamma(a')$, where $c' \subseteq \gamma(a')$. Since $f^\sharp_2$ is sound, $f_2(c') \subseteq \gamma(f^\sharp_2(a'))$. 
% Hence $f^\sharp_1 \circ f^\sharp_2$ is sound.
% \end{proof}
\begin{proof}
    Let $c\subseteq \gamma(a)$ \\ 
    Since $f_1^\sharp$ is sound w.r.t $f_1$, $f_1(c) \subseteq \gamma(f_1^\sharp(a))$ \\ 
    Let $c_2 = f_1(c)$ and $a_2 = f_1^\sharp(a)$ \\ 
    $\implies c_2 \subseteq \gamma(a_2)$ \\ 
    Since $f_2^\sharp$ is sound w.r.t $f_2$, $f_2(c_2) \subseteq \gamma(f_2^\sharp(a_2))$ \\ 
    $\implies f_2(f_1(c)) \subseteq \gamma(f_2^\sharp(f_1^\sharp(a)))$ \\
    Hence, $f_1^\sharp \circ f_2^\sharp$ is sound w.r.t $f_1 \circ f_2$
\end{proof}
